# Supplementary material for: Tag loss models for capture-recapture data without double tagging
Source: arXiv:2610.30447 source file (2026-10-21)
Supplement: Supplementary file 1 [file supplementary_material.tex]

\section{Supplementary Material}\label{supp_mat}
